# Supplementary material for: Pair Correlation Functions of Strongly Coupled Two-Temperature Plasma
Source: arXiv:1707.01509 ancillary file (2017-07-05)

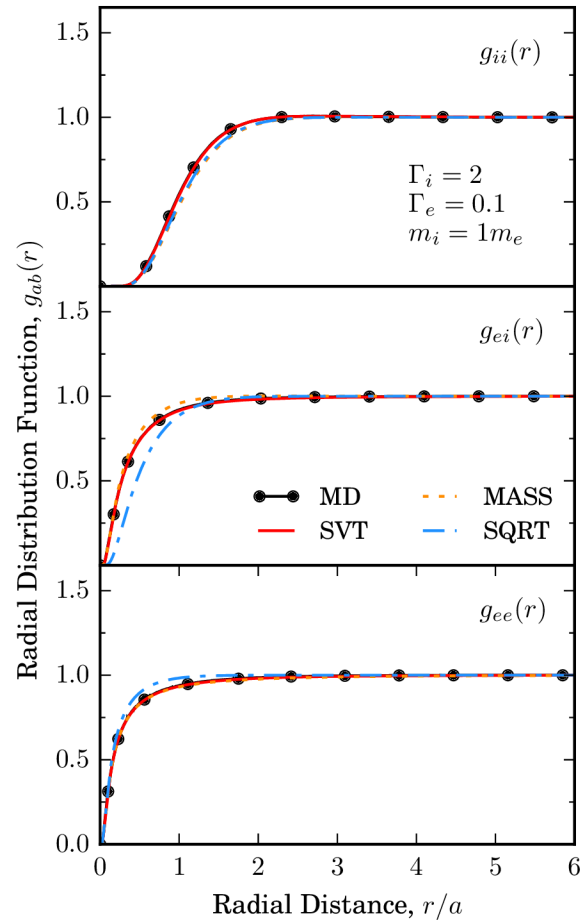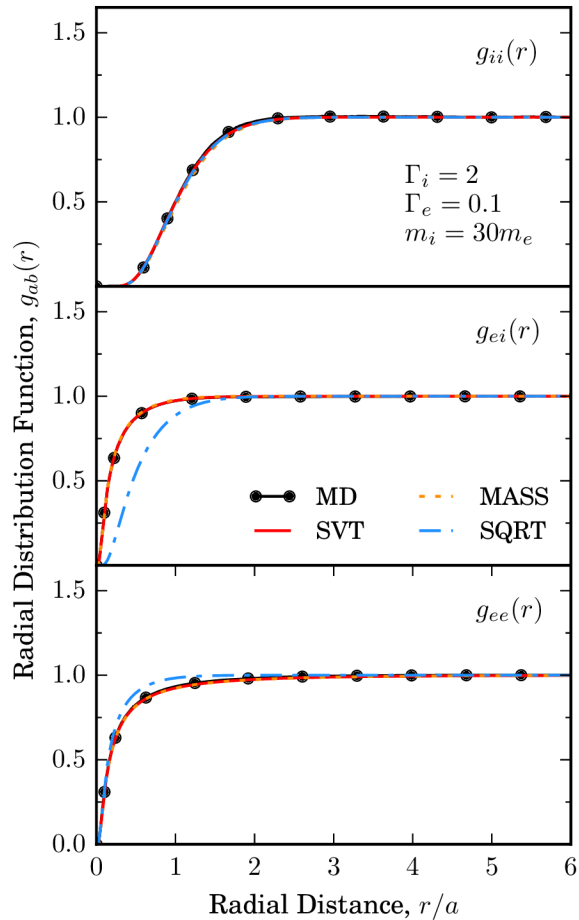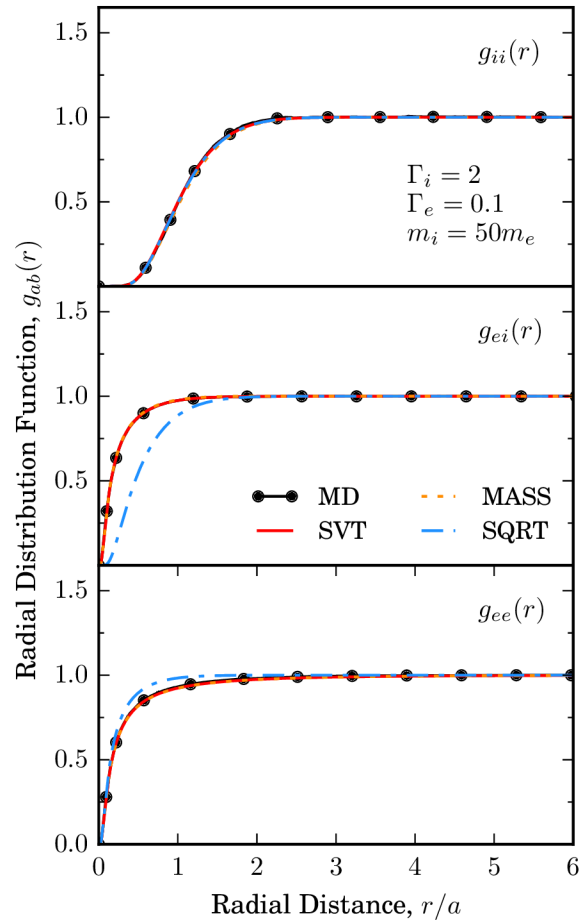

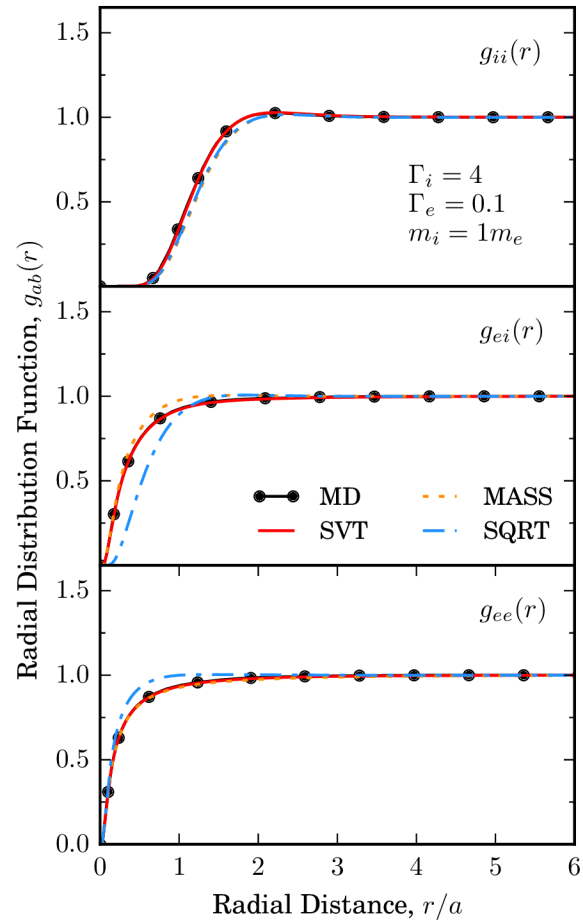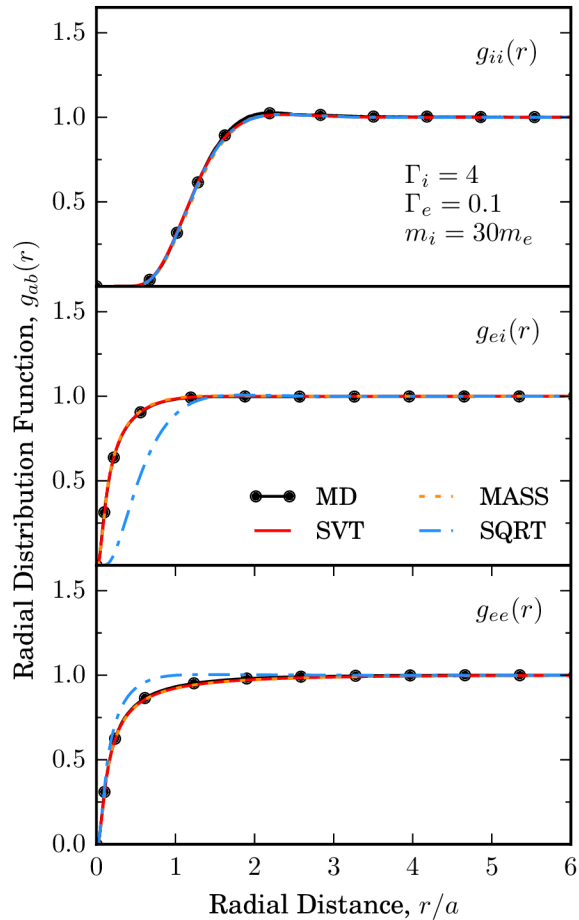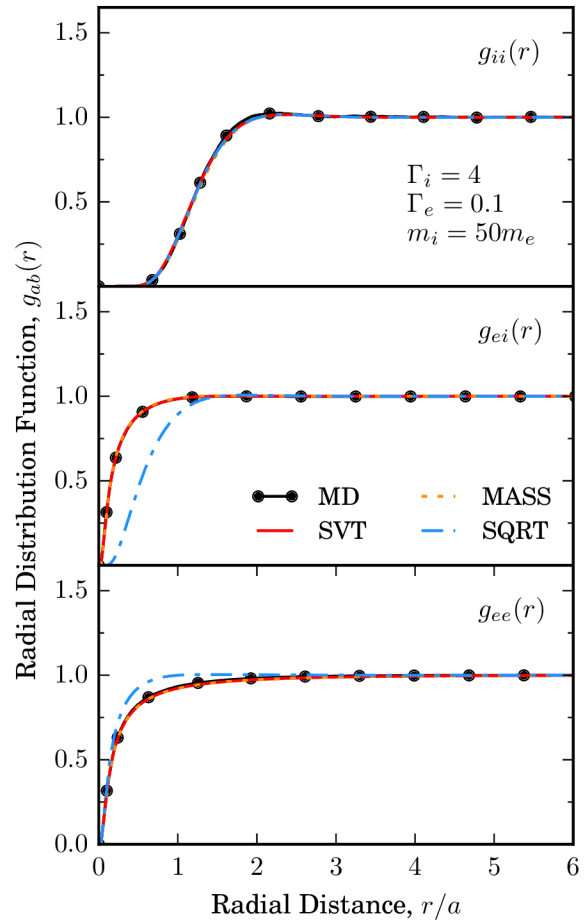

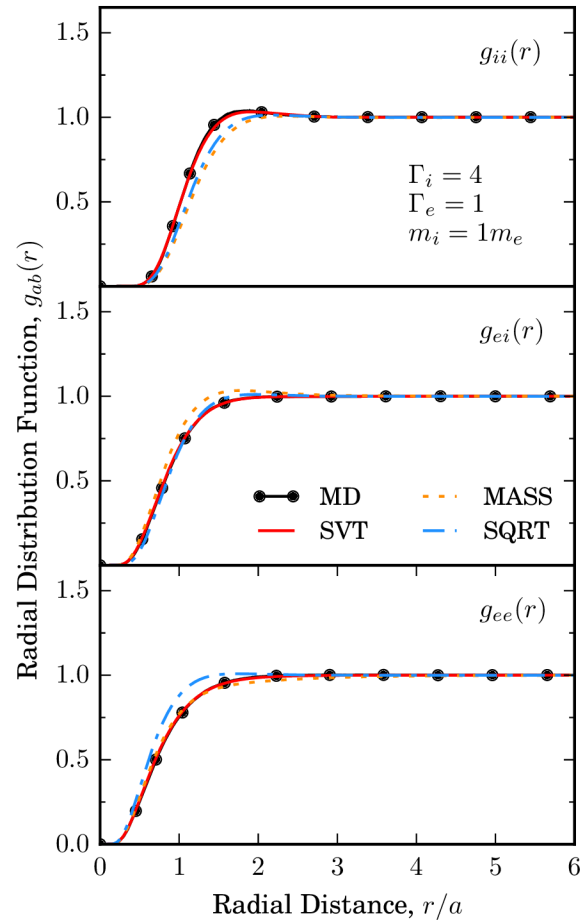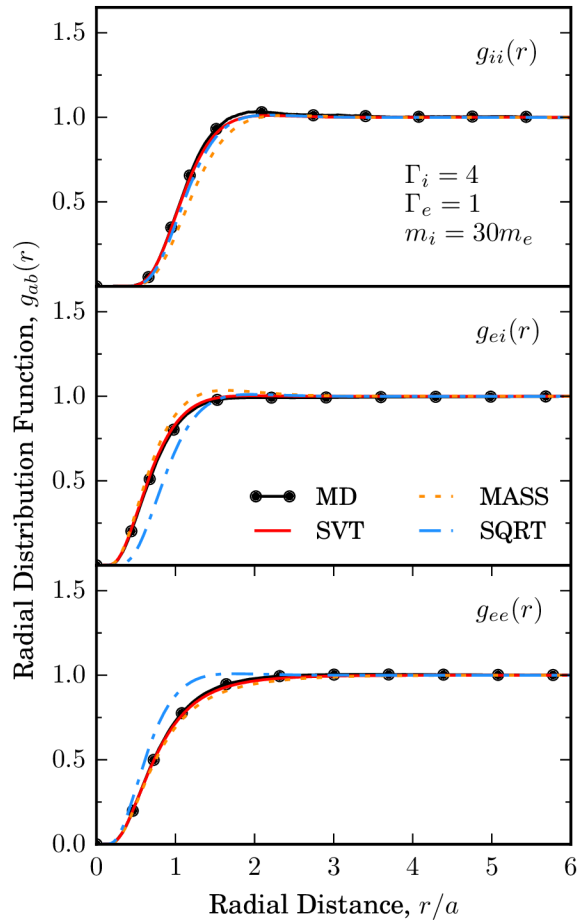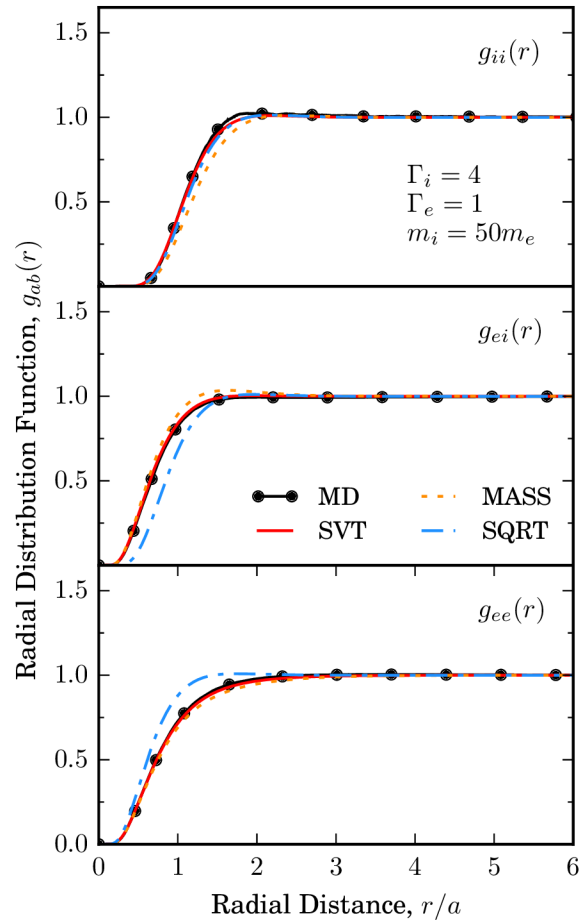

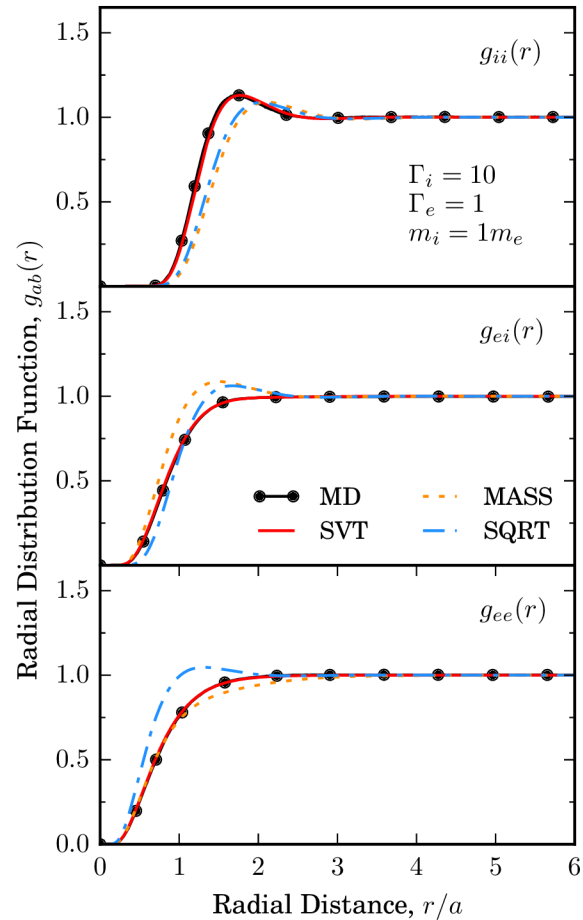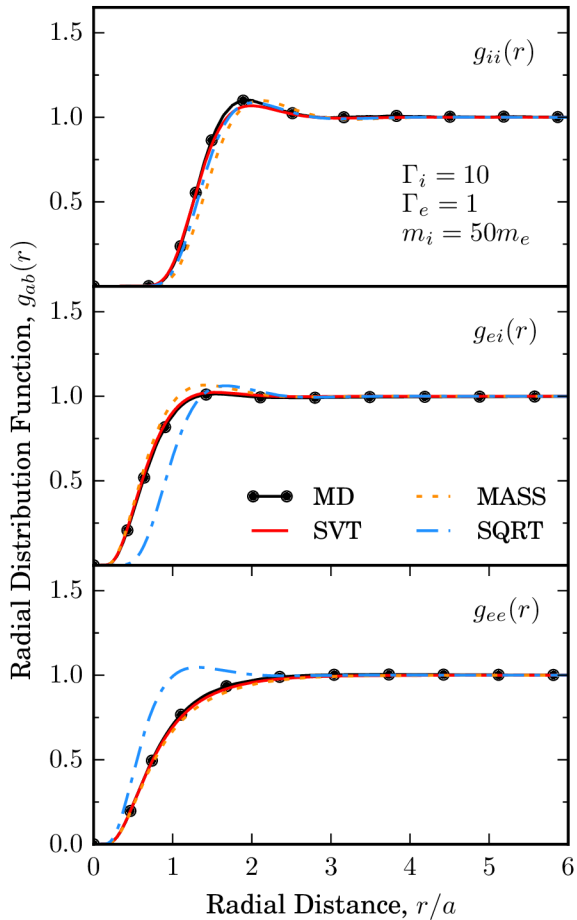

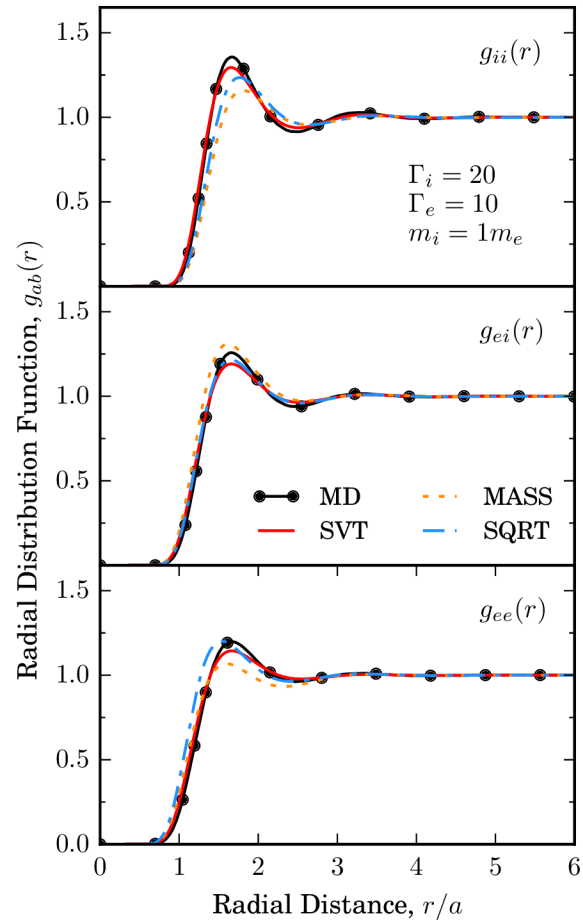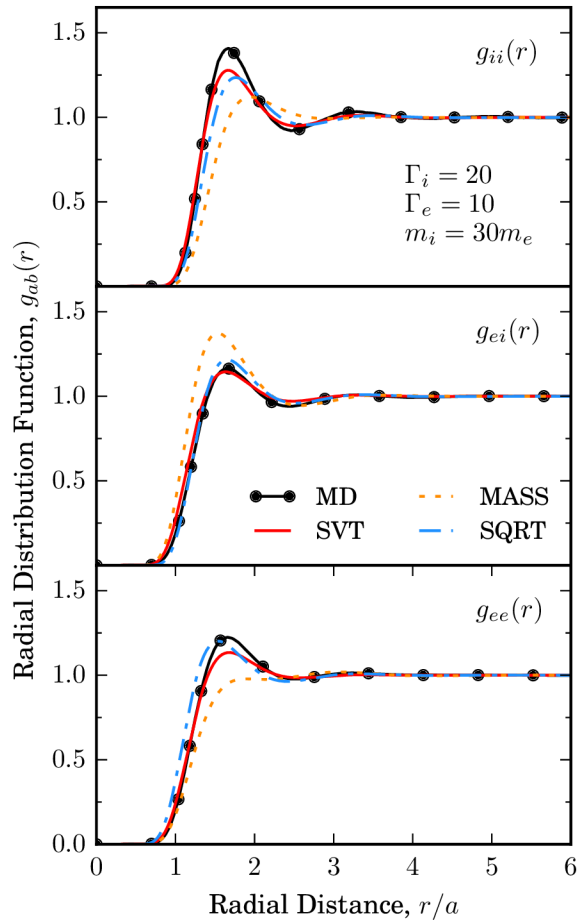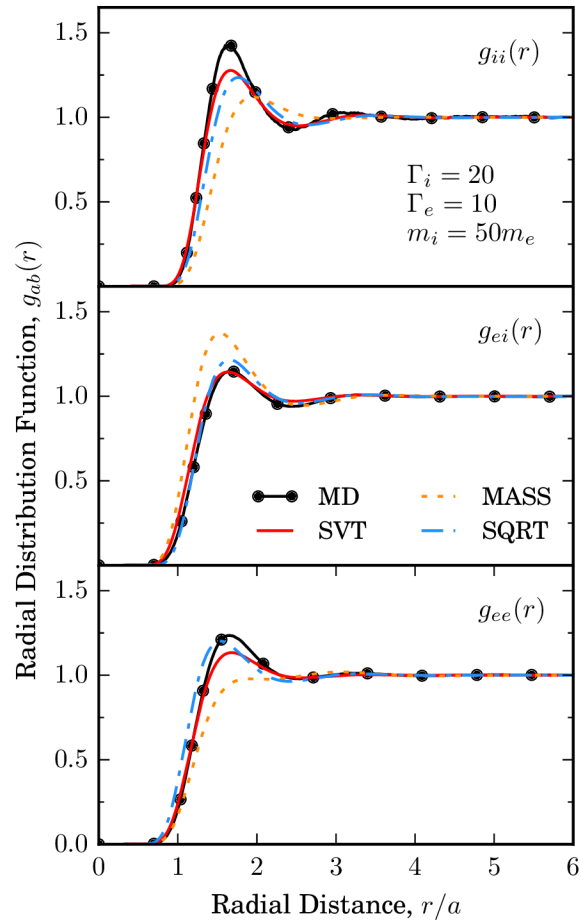

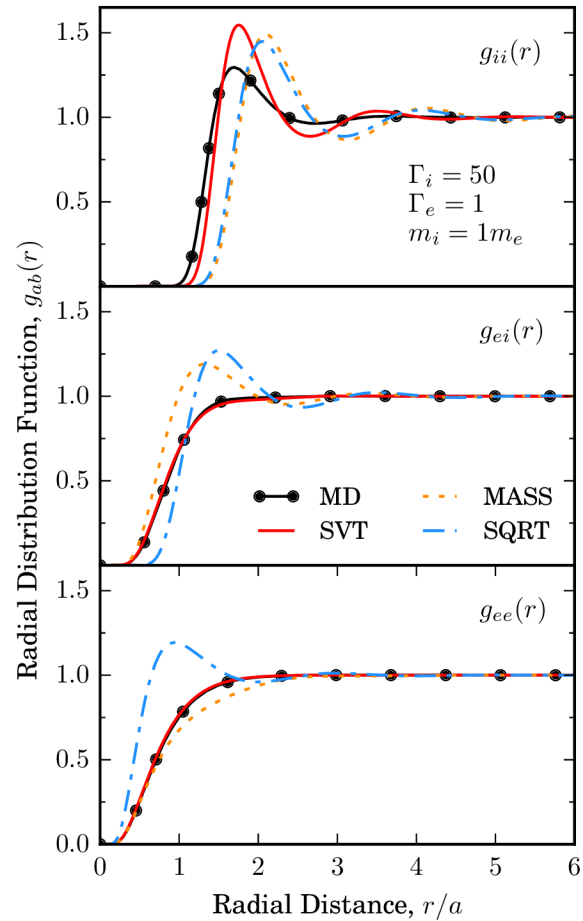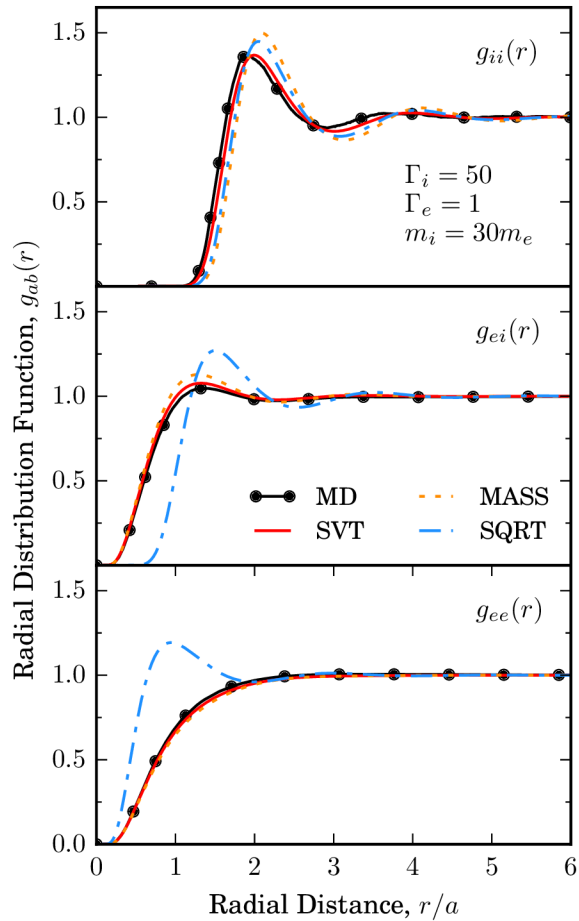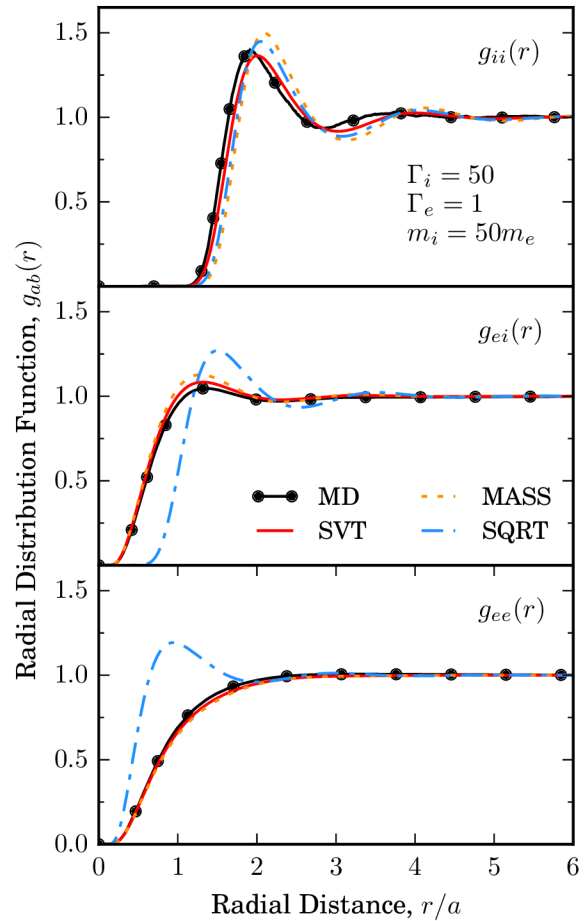

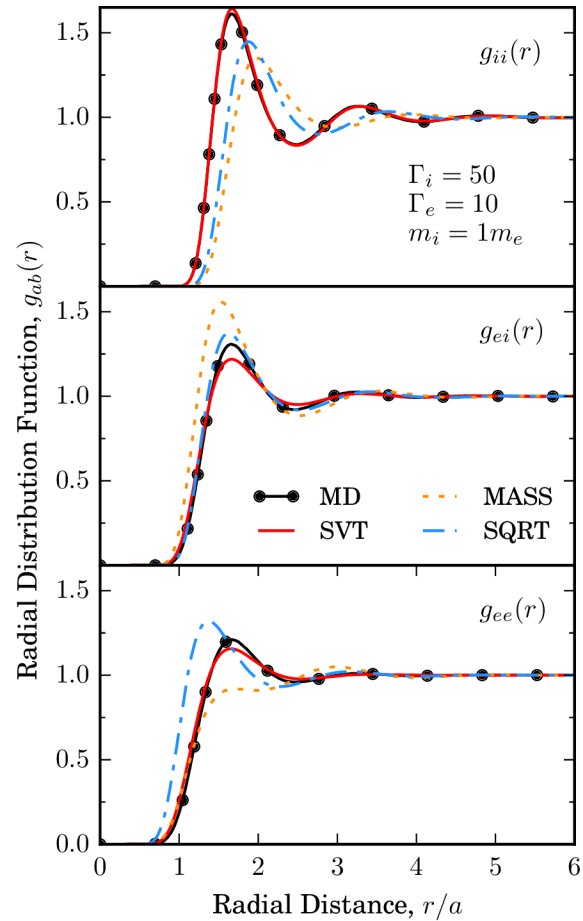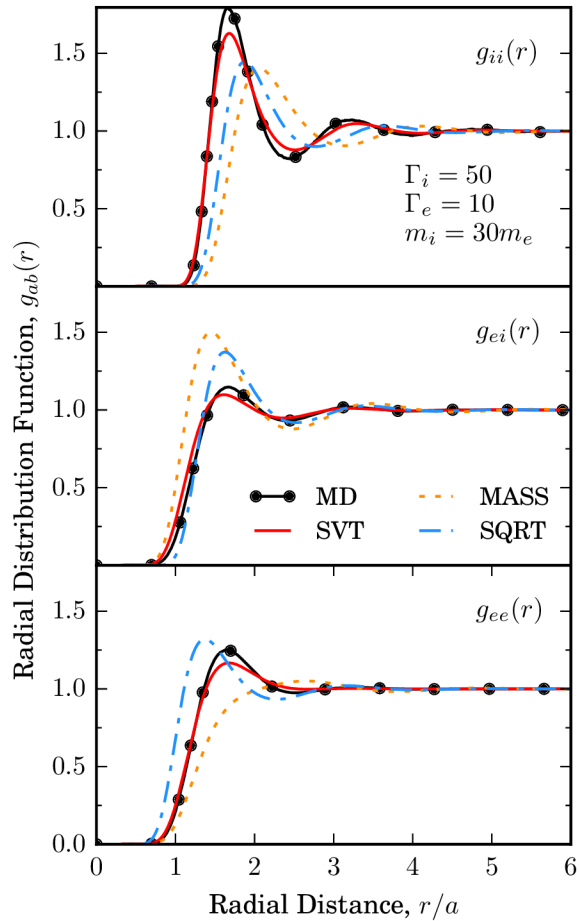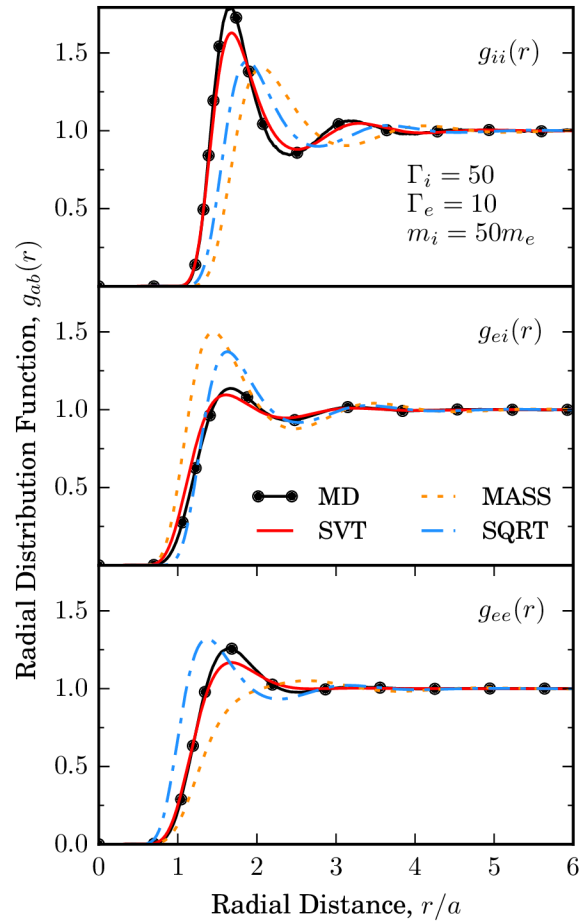

Supplement: Supplementary file 2 [file gr_all.pdf]
